# Supplementary material for: A Practical and Secure Byzantine Robust Aggregator
Source: arXiv:2506.23183 source file (2025-10-12)
Supplement: Supplementary file 1 [file appendix_scheduler.tex]

\section{\randeigen with Power Iteration Scheduler} \label{appendix:power_iter_schedule}

We investigate the use of a scheduler to accelerate the power iteration portion in \randeigen
(Section \ref{subsection:power_iter}).
This is implemented as the following: Let $\lambda_i$ be the
dominant eigenvalue computed in the $i$-th iteration, where $i \geq 1$, and $\epsilon_P$ denote
the initial error rate for the power iteration. 
\begin{enumerate}
    \item For each iteration $i > 1$, let $\Delta_i = 1-\lambda_i/\lambda_{i-1}$ be the
    percentage drop in the dominant  eigenvalue from the $i-1$ to $i$ iteration. 
    \item Scale $\epsilon_P = \Delta_i \times \epsilon_P$.
\end{enumerate}

The intuition behind the scheduler is as follows: 
In the initial filtering rounds, where the dataset contains more poisoned samples, 
a coarse approximation of the sample projections on the dominant eigenvector is sufficient,
which requires fewer iterations. Therefore, we dynamically scale $\epsilon_P$ based on 
the reduction in eigenvalue between successive iterations. This intuition is similar to
other dynamic schedulers employed in machine learning.

\begin{table*}[]
\caption{Evaluation of \randeigen with a scheduler incorporated, with an average speedup of approximately 18.1\%}
\label{table:randeigen_scheduler}
\begin{tabular}{|l|l|l|cccccc|l|}
\hline
\multicolumn{1}{|c|}{\multirow{3}{*}{Type}} & \multicolumn{1}{c|}{\multirow{3}{*}{Attack}} & \multicolumn{1}{c|}{\multirow{3}{*}{Dataset}} & \multicolumn{6}{c|}{\randeigen}                                                   & \multicolumn{1}{c|}{\multirow{3}{*}{Speedup (\%)}} \\ \cline{4-9}
\multicolumn{1}{|c|}{}                      & \multicolumn{1}{c|}{}                        & \multicolumn{1}{c|}{}                         & \multicolumn{3}{c|}{No Scheduler}           & \multicolumn{3}{c|}{With Scheduler} & \multicolumn{1}{c|}{}                             \\ \cline{4-9}
\multicolumn{1}{|c|}{}                      & \multicolumn{1}{c|}{}                        & \multicolumn{1}{c|}{}                         & ASR    & ACC    & \multicolumn{1}{c|}{Time} & ASR         & ACC        & Time     & \multicolumn{1}{c|}{}                             \\ \hline
\multicolumn{1}{|c|}{\multirow{2}{*}{-}}    & \multirow{2}{*}{No Attack}                   & MNIST                                         & -      & 94.5\% & \multicolumn{1}{c|}{2.48} & -           & 92.7\%     & 1.99     & 19.76                                             \\
\multicolumn{1}{|c|}{}                      &                                              & F-MNIST                                       & -      & 81.1\% & \multicolumn{1}{c|}{2.33} & -           & 81.0\%     & 2.01     & 13.73                                             \\ \hline
\multirow{4}{*}{Backdoor}                   & \multirow{2}{*}{MRA}                         & MNIST                                         & 5.4\%  & 92.4\% & \multicolumn{1}{c|}{2.42} & 6.1\%       & 93.7\%     & 1.81     & 25.21                                             \\
                                            &                                              & F-MNIST                                       & 10.0\% & 76.1\% & \multicolumn{1}{c|}{2.16} & 10.0\%      & 77.0\%     & 2.00     & 7.41                                              \\ \cline{2-10} 
                                            & \multirow{2}{*}{DBA}                         & MNIST                                         & 3.1\%  & 93.1\% & \multicolumn{1}{c|}{2.40} & 4.0\%       & 91.9\%     & 1.78     & 25.83                                             \\
                                            &                                              & F-MNIST                                       & 14.0\% & 78.4\% & \multicolumn{1}{c|}{2.78} & 11.0\%      & 78.0\%     & 2.08     & 25.18                                             \\ \hline
\multirow{2}{*}{Targeted}                   & \multirow{2}{*}{MPA}                         & MNIST                                         & 10.0\% & 95.0\% & \multicolumn{1}{c|}{2.32} & 10.0\%      & 94.1\%     & 1.85     & 20.26                                             \\
                                            &                                              & F-MNIST                                       & 10.0\% & 79.8\% & \multicolumn{1}{c|}{2.38} & 10.0\%      & 77.9\%     & 1.99     & 16.39                                             \\ \hline
\multirow{4}{*}{Untargeted}                 & \multirow{2}{*}{HIDRA}                       & MNIST                                         & -      & 93.4\% & \multicolumn{1}{c|}{2.10} & -           & 90.4\%     & 2.02     & 3.81                                              \\
                                            &                                              & F-MNIST                                       & -      & 76.8\% & \multicolumn{1}{c|}{2.21} & -           & 74.1\%     & 1.90     & 14.03                                             \\ \cline{2-10} 
                                            & \multirow{2}{*}{TMA}                         & MNIST                                         & -      & 94.1\% & \multicolumn{1}{c|}{2.57} & -           & 93.2\%     & 1.83     & 28.79                                             \\
                                            &                                              & F-MNIST                                       & -      & 77.8\% & \multicolumn{1}{c|}{2.41} & -           & 79.8\%     & 2.00     & 17.01                                             \\ \hline
\end{tabular}
\end{table*}

We evaluated the power iteration scheduler scheme on the image classification tasks, with an initial $\epsilon_P = 0.5$. The evaluation results are reported in 
Table \ref{table:randeigen_scheduler}. 

% \begin{algorithm}[t]
% \caption{Pseudo-code describing Power Iteration Scheduler}
% % \label{alg:filter_modified}
% \begin{algorithmic}[1] % Set the line numbering to start at 1
% % \REQUIRE Input data
% % \ENSURE Output data 
% \REQUIRE Current power iteration error rate $\epsilon_P$, 
% $$
% \ENSURE Robust aggregate $\mu = \{\mu_1, \dots, \mu_n\}$, where $\mu_i$ is the robust aggregate of the $i$-th dimension

% \FOR{$j=1$ {\bfseries to} $ n \cdot \epsilon$} 
%     \STATEx \quad $\triangleright$  Obtain dominant eigenvalue/vector
%     \STATE $\lambda_{curr}, u := EIGENDECOMPOSITION(Cov(X))$ 
%     \STATEx \quad $\triangleright$  Eigenvalue has converged
%     \IF{$j > 1$ \bf{and} $\lambda_{curr} \stackrel{f}{=}  \lambda_{old}$} \label{algo:stop}
%          break
%     \ELSE
%         \STATE $\lambda_{old}  = \lambda_{curr}$
%     \ENDIF
%     \STATE $\mu_x = \frac{1}{|X|} \sum_{x \in X} x$
%     \STATE  $\mathcal{P} = \{p_1, \dots, p_n\}$, where $p_i = |\langle X_i, u \rangle -  \langle \mu_x, u  \rangle|$
%     \FOR {$i= 1$ {\bfseries to} $ |X|$} 
%         \STATE Remove $x_i$ from $X$ with probability $p_i / \max \mathcal{P}$
%     \ENDFOR
% \ENDFOR
% \State \textbf{return} $\mu$ = Dimension-wise average of $X$
% \end{algorithmic}
% \end{algorithm}
