# Supplementary material for: A Practical and Secure Byzantine Robust Aggregator
Source: arXiv:2506.23183 source file (2025-10-12)
Supplement: Supplementary file 2 [file appendix_new_expt.tex]

\section{Additional Experiments}
